# Supplementary material for: Augmenting Sheet Music with Rhythmic Fingerprints
Source: arXiv:2009.02057 source file (2020-09-04)
Supplement: Supplementary file 1 [file Goldberg_Variations_-_Johann_Sebastian_Bach_-_Aria_MS1_with_Fingerprints_optimiert.pdf]

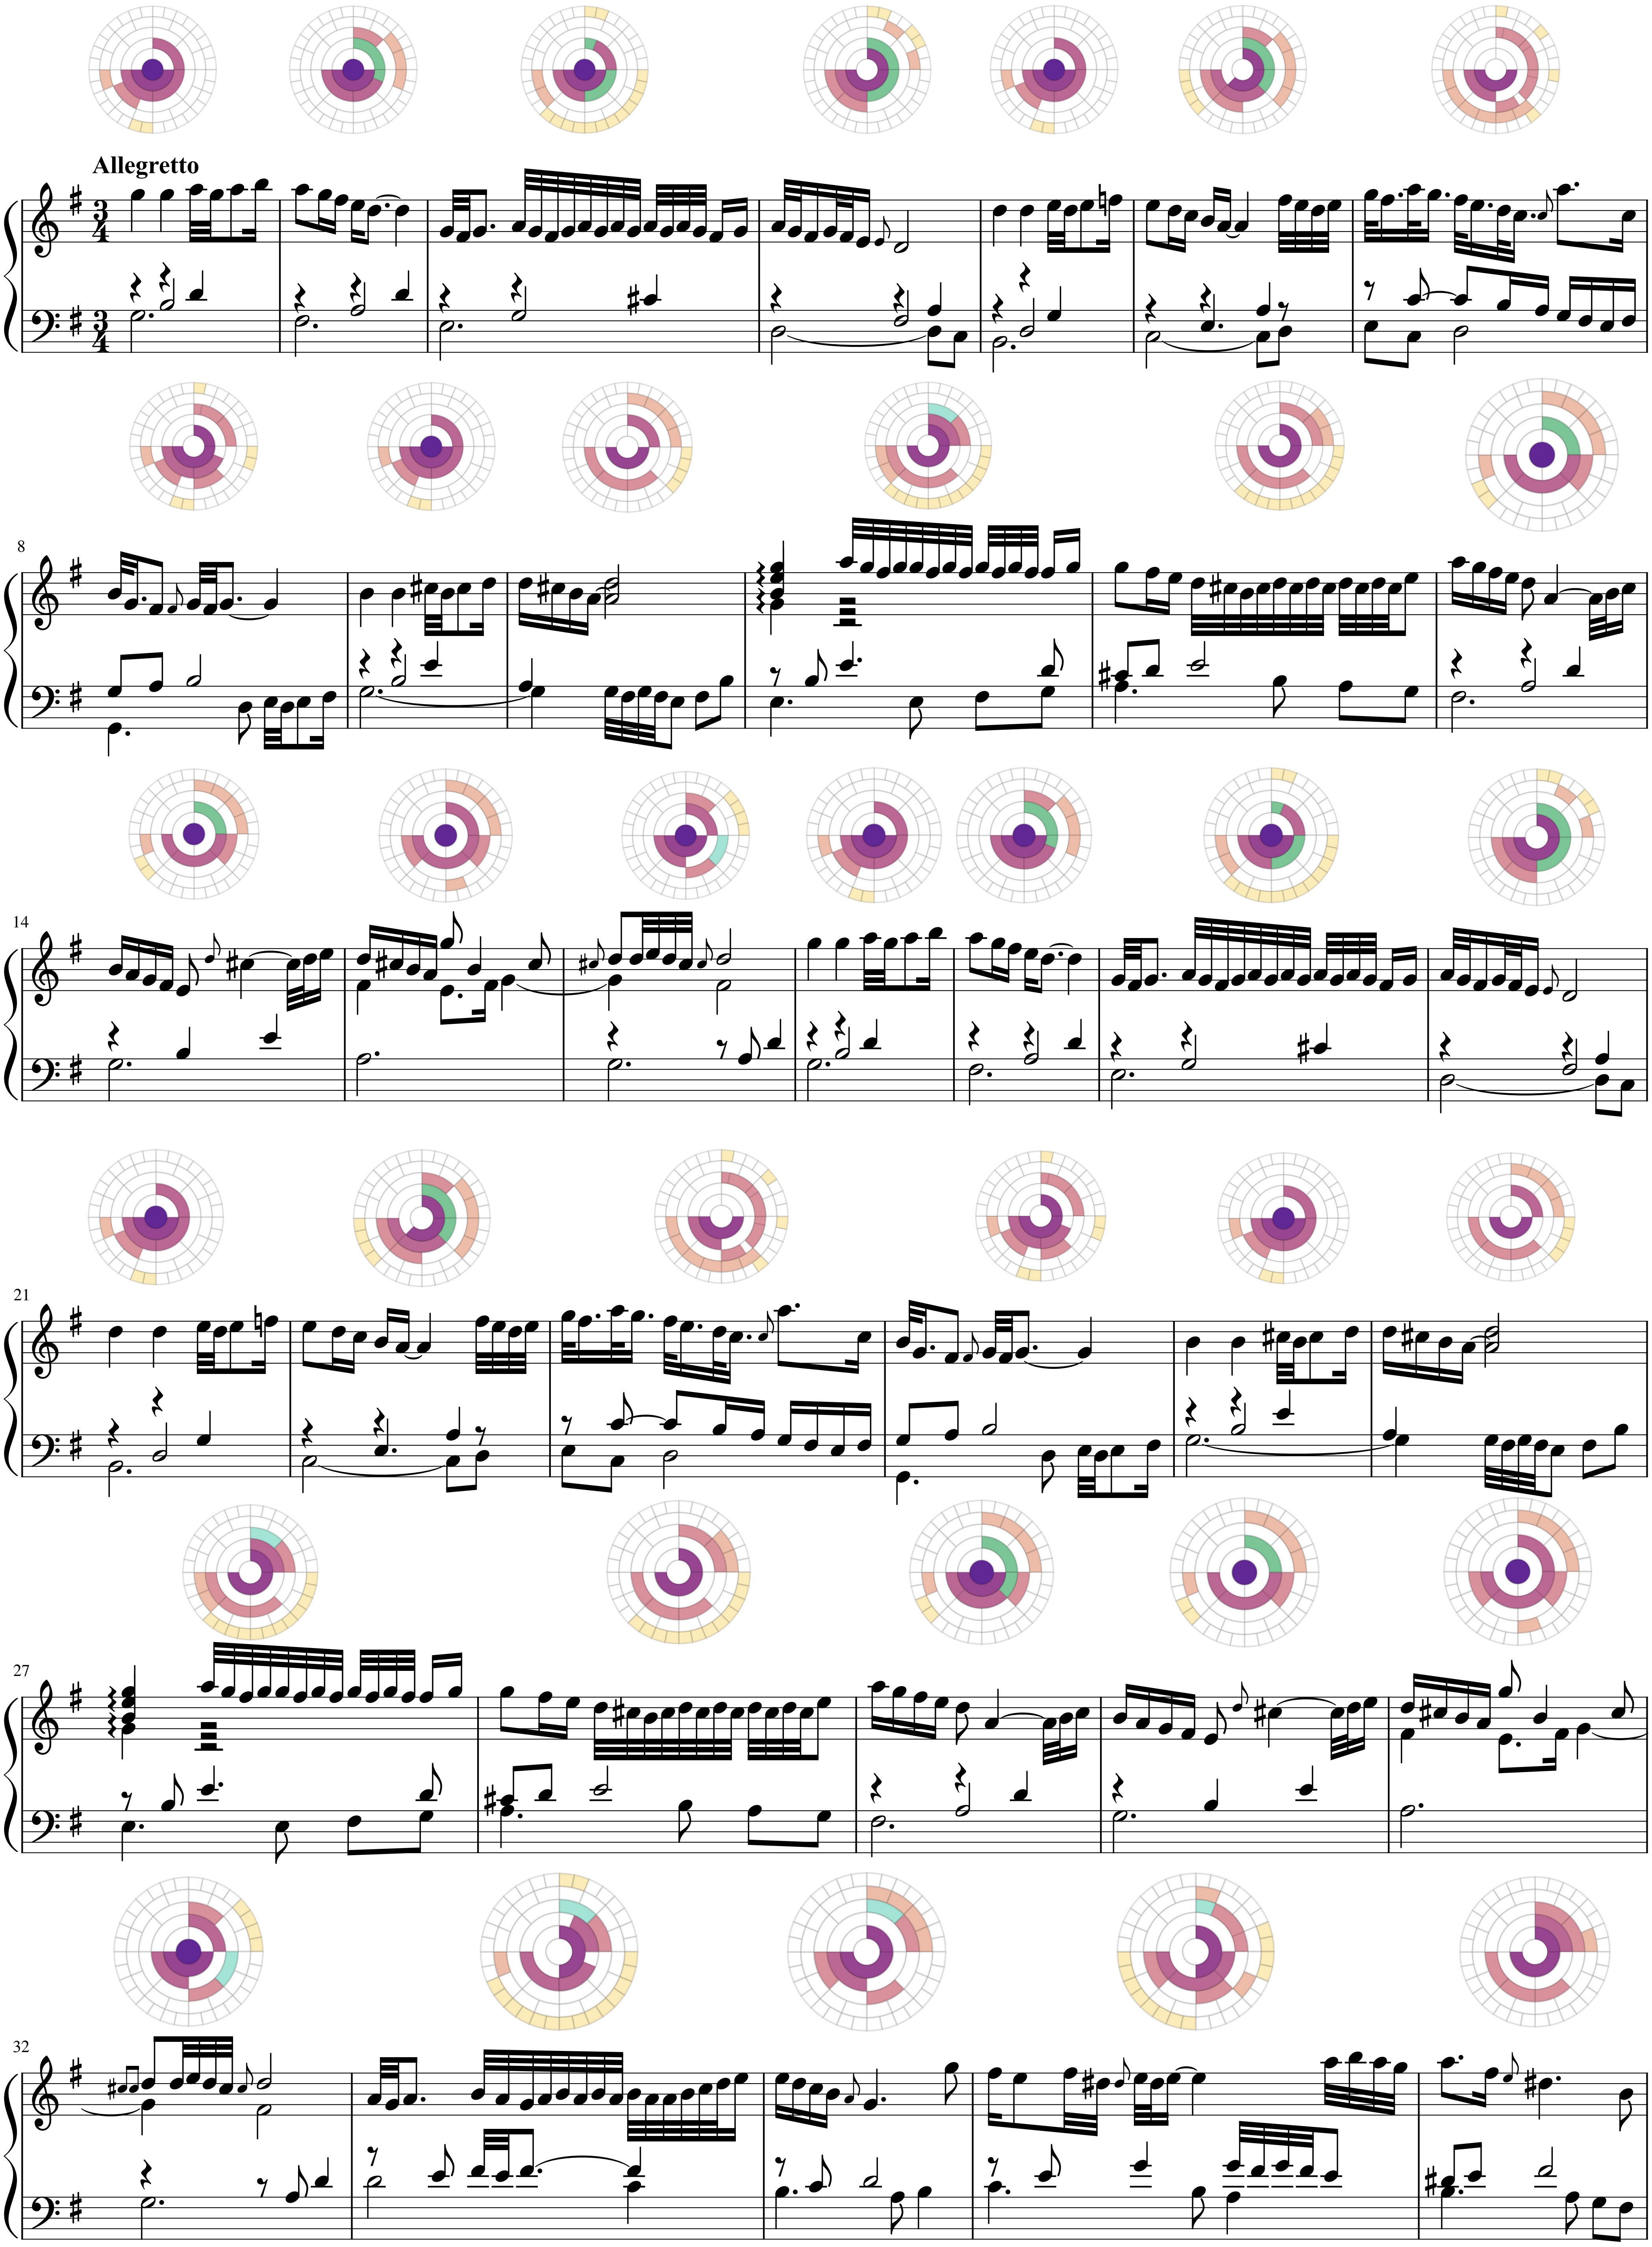
Allegretto

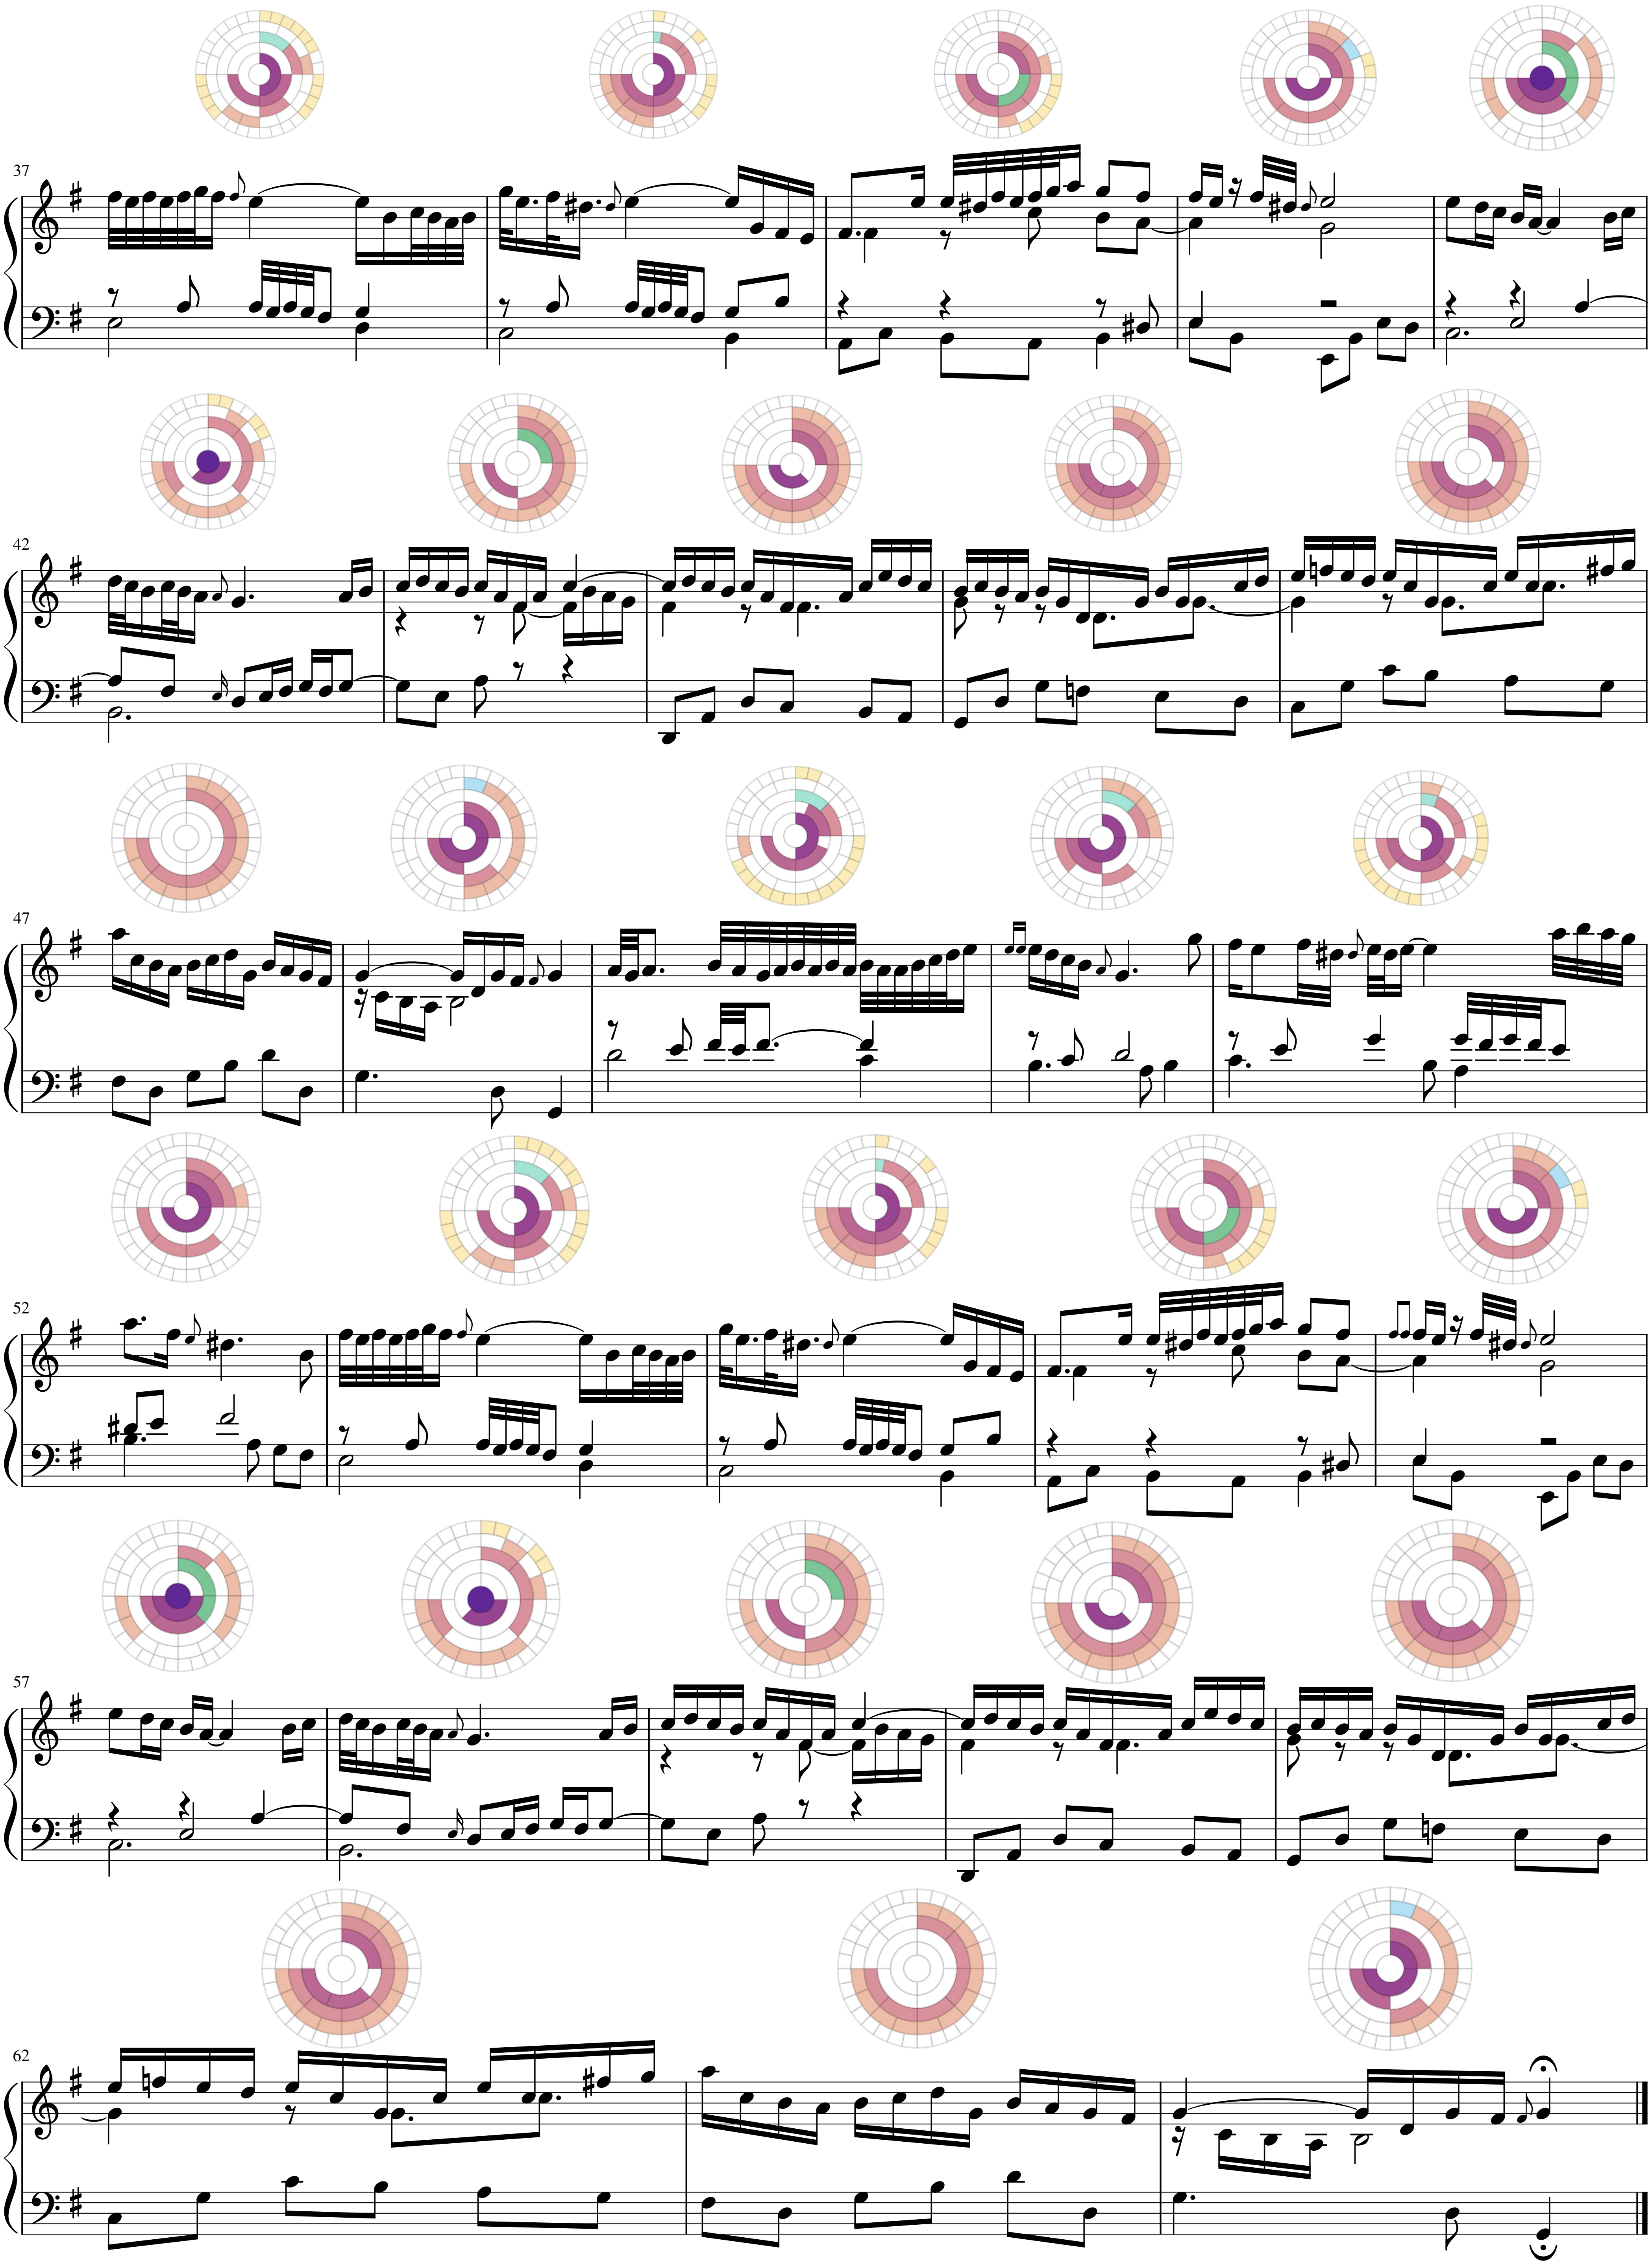
37
42
47
52
57
62
