# Supplementary material for: Augmenting Sheet Music with Rhythmic Fingerprints
Source: arXiv:2009.02057 source file (2020-09-04)
Supplement: Supplementary file 2 [file Goldberg_Variations_-_Johann_Sebastian_Bach_-_Variation_VII_MS2_with_Fingerprints_optimiert.pdf]

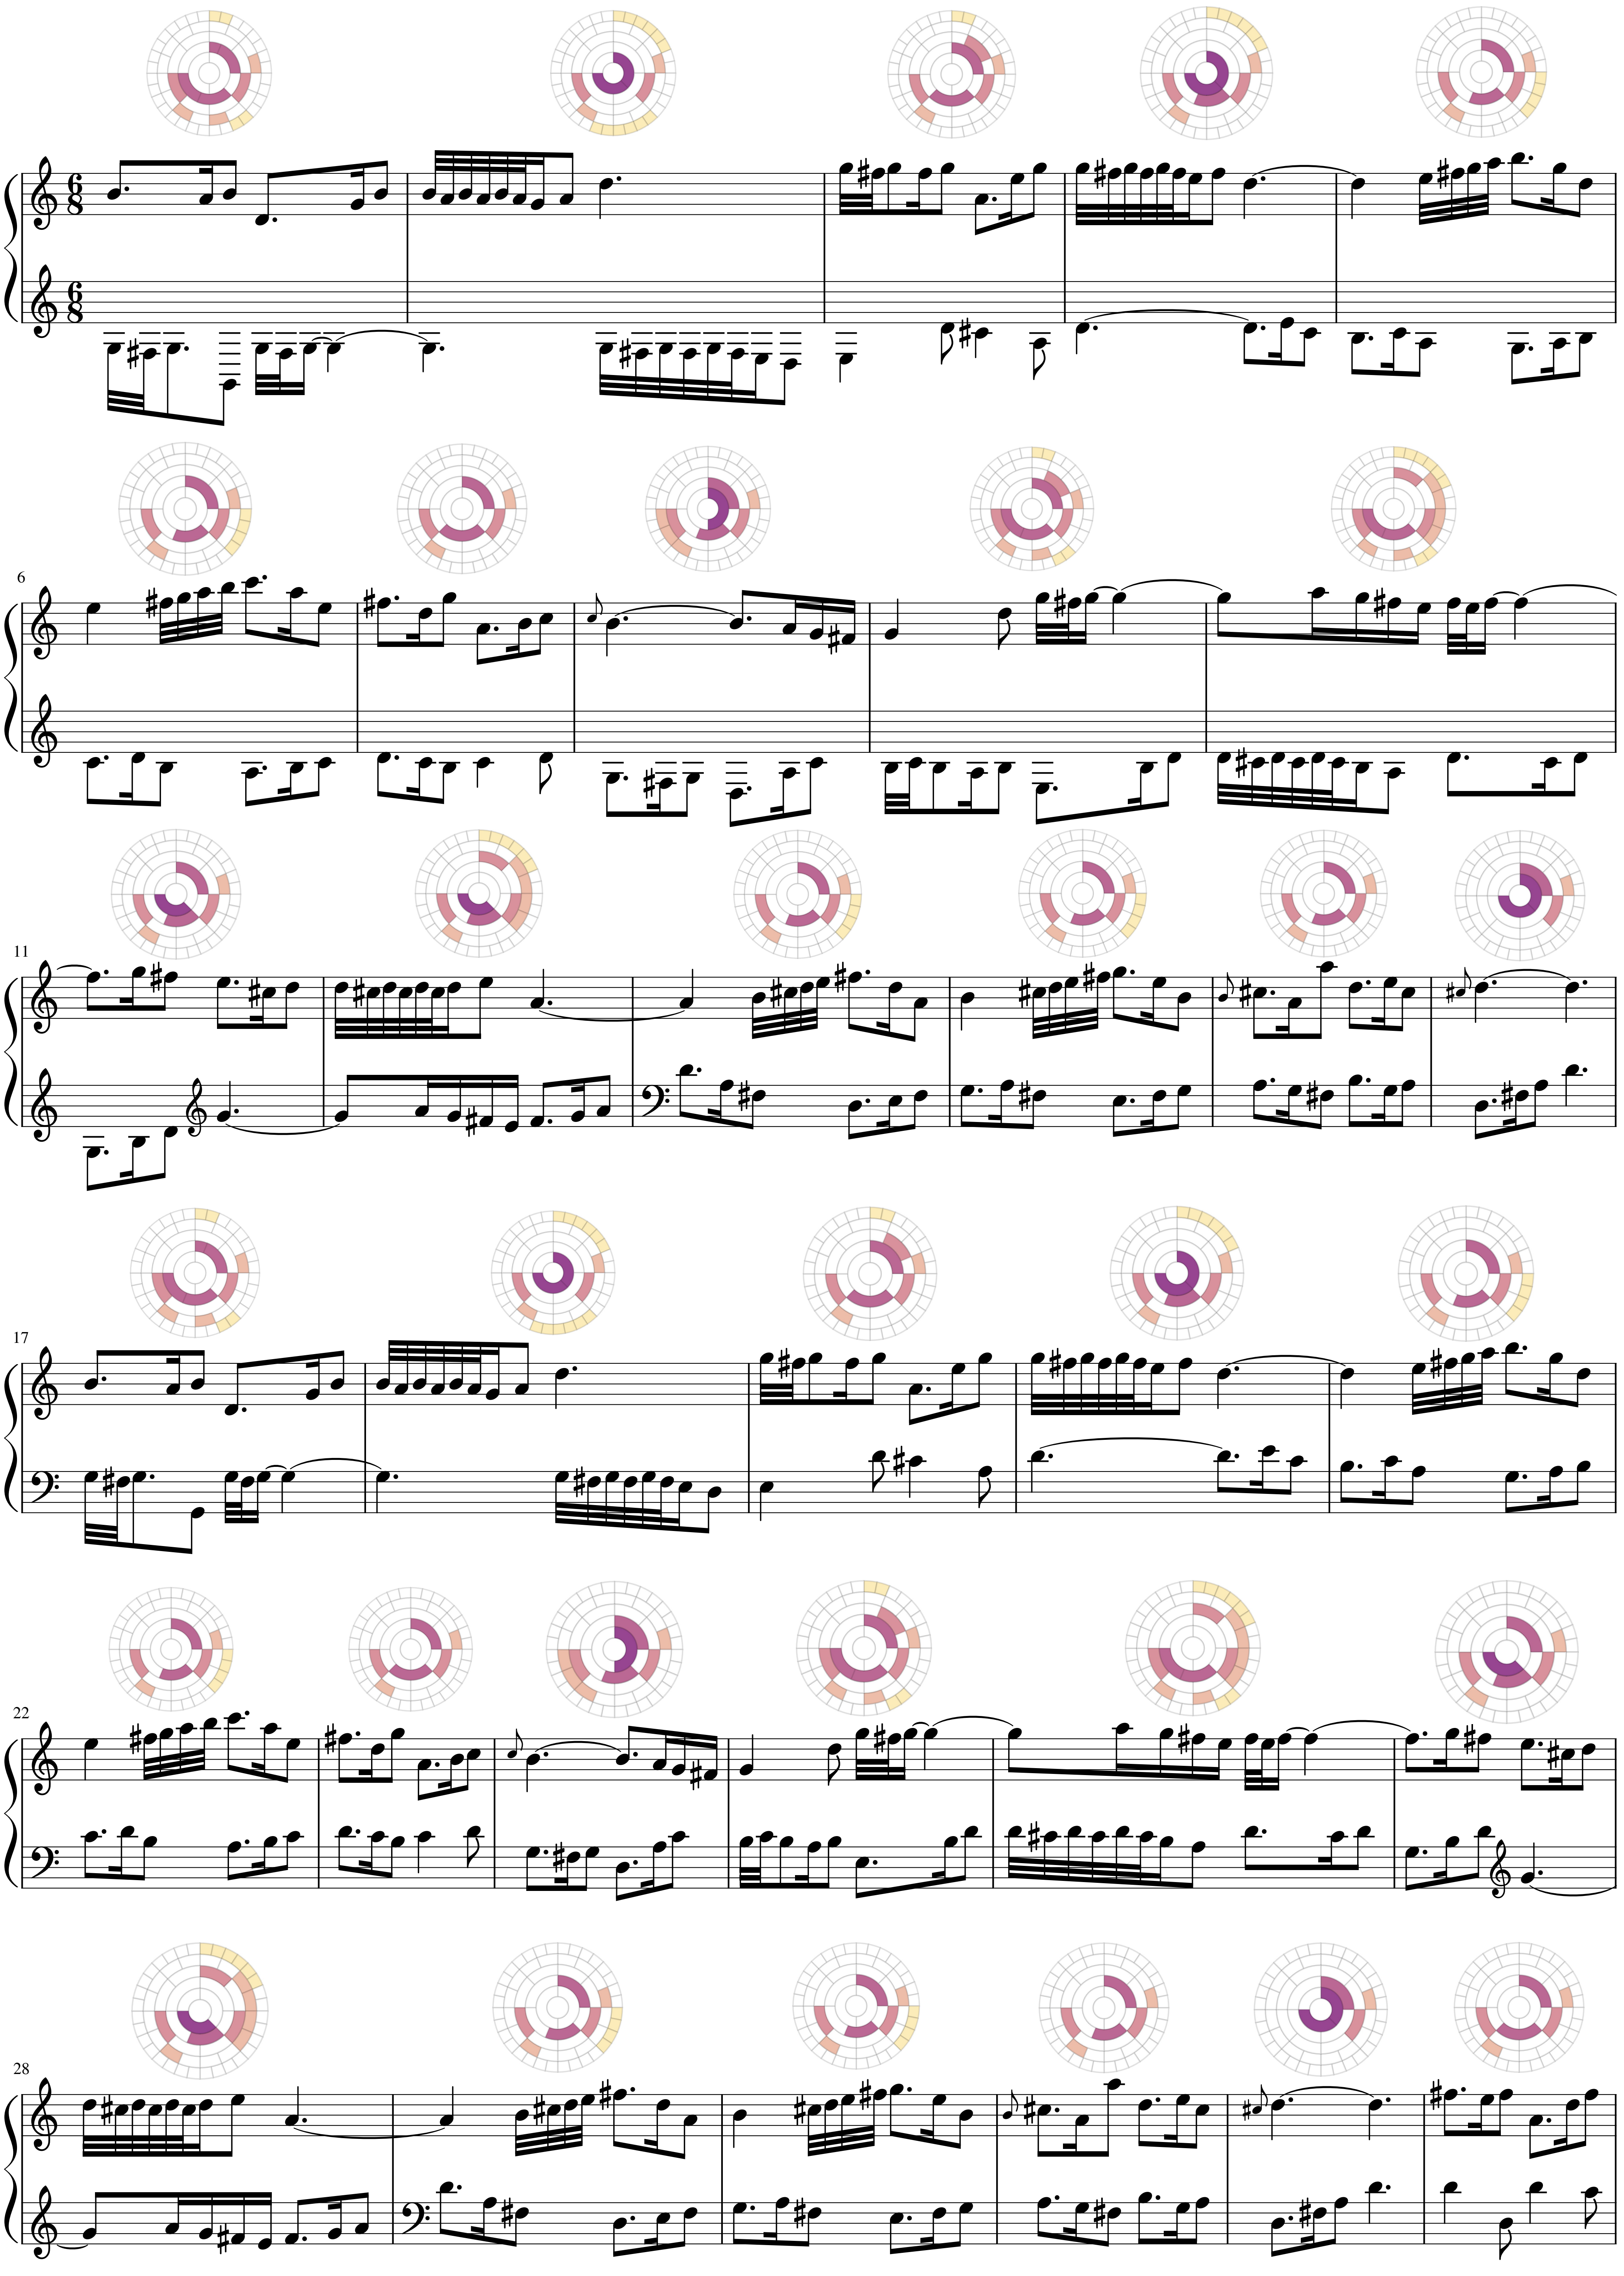
6
11
17
22
28

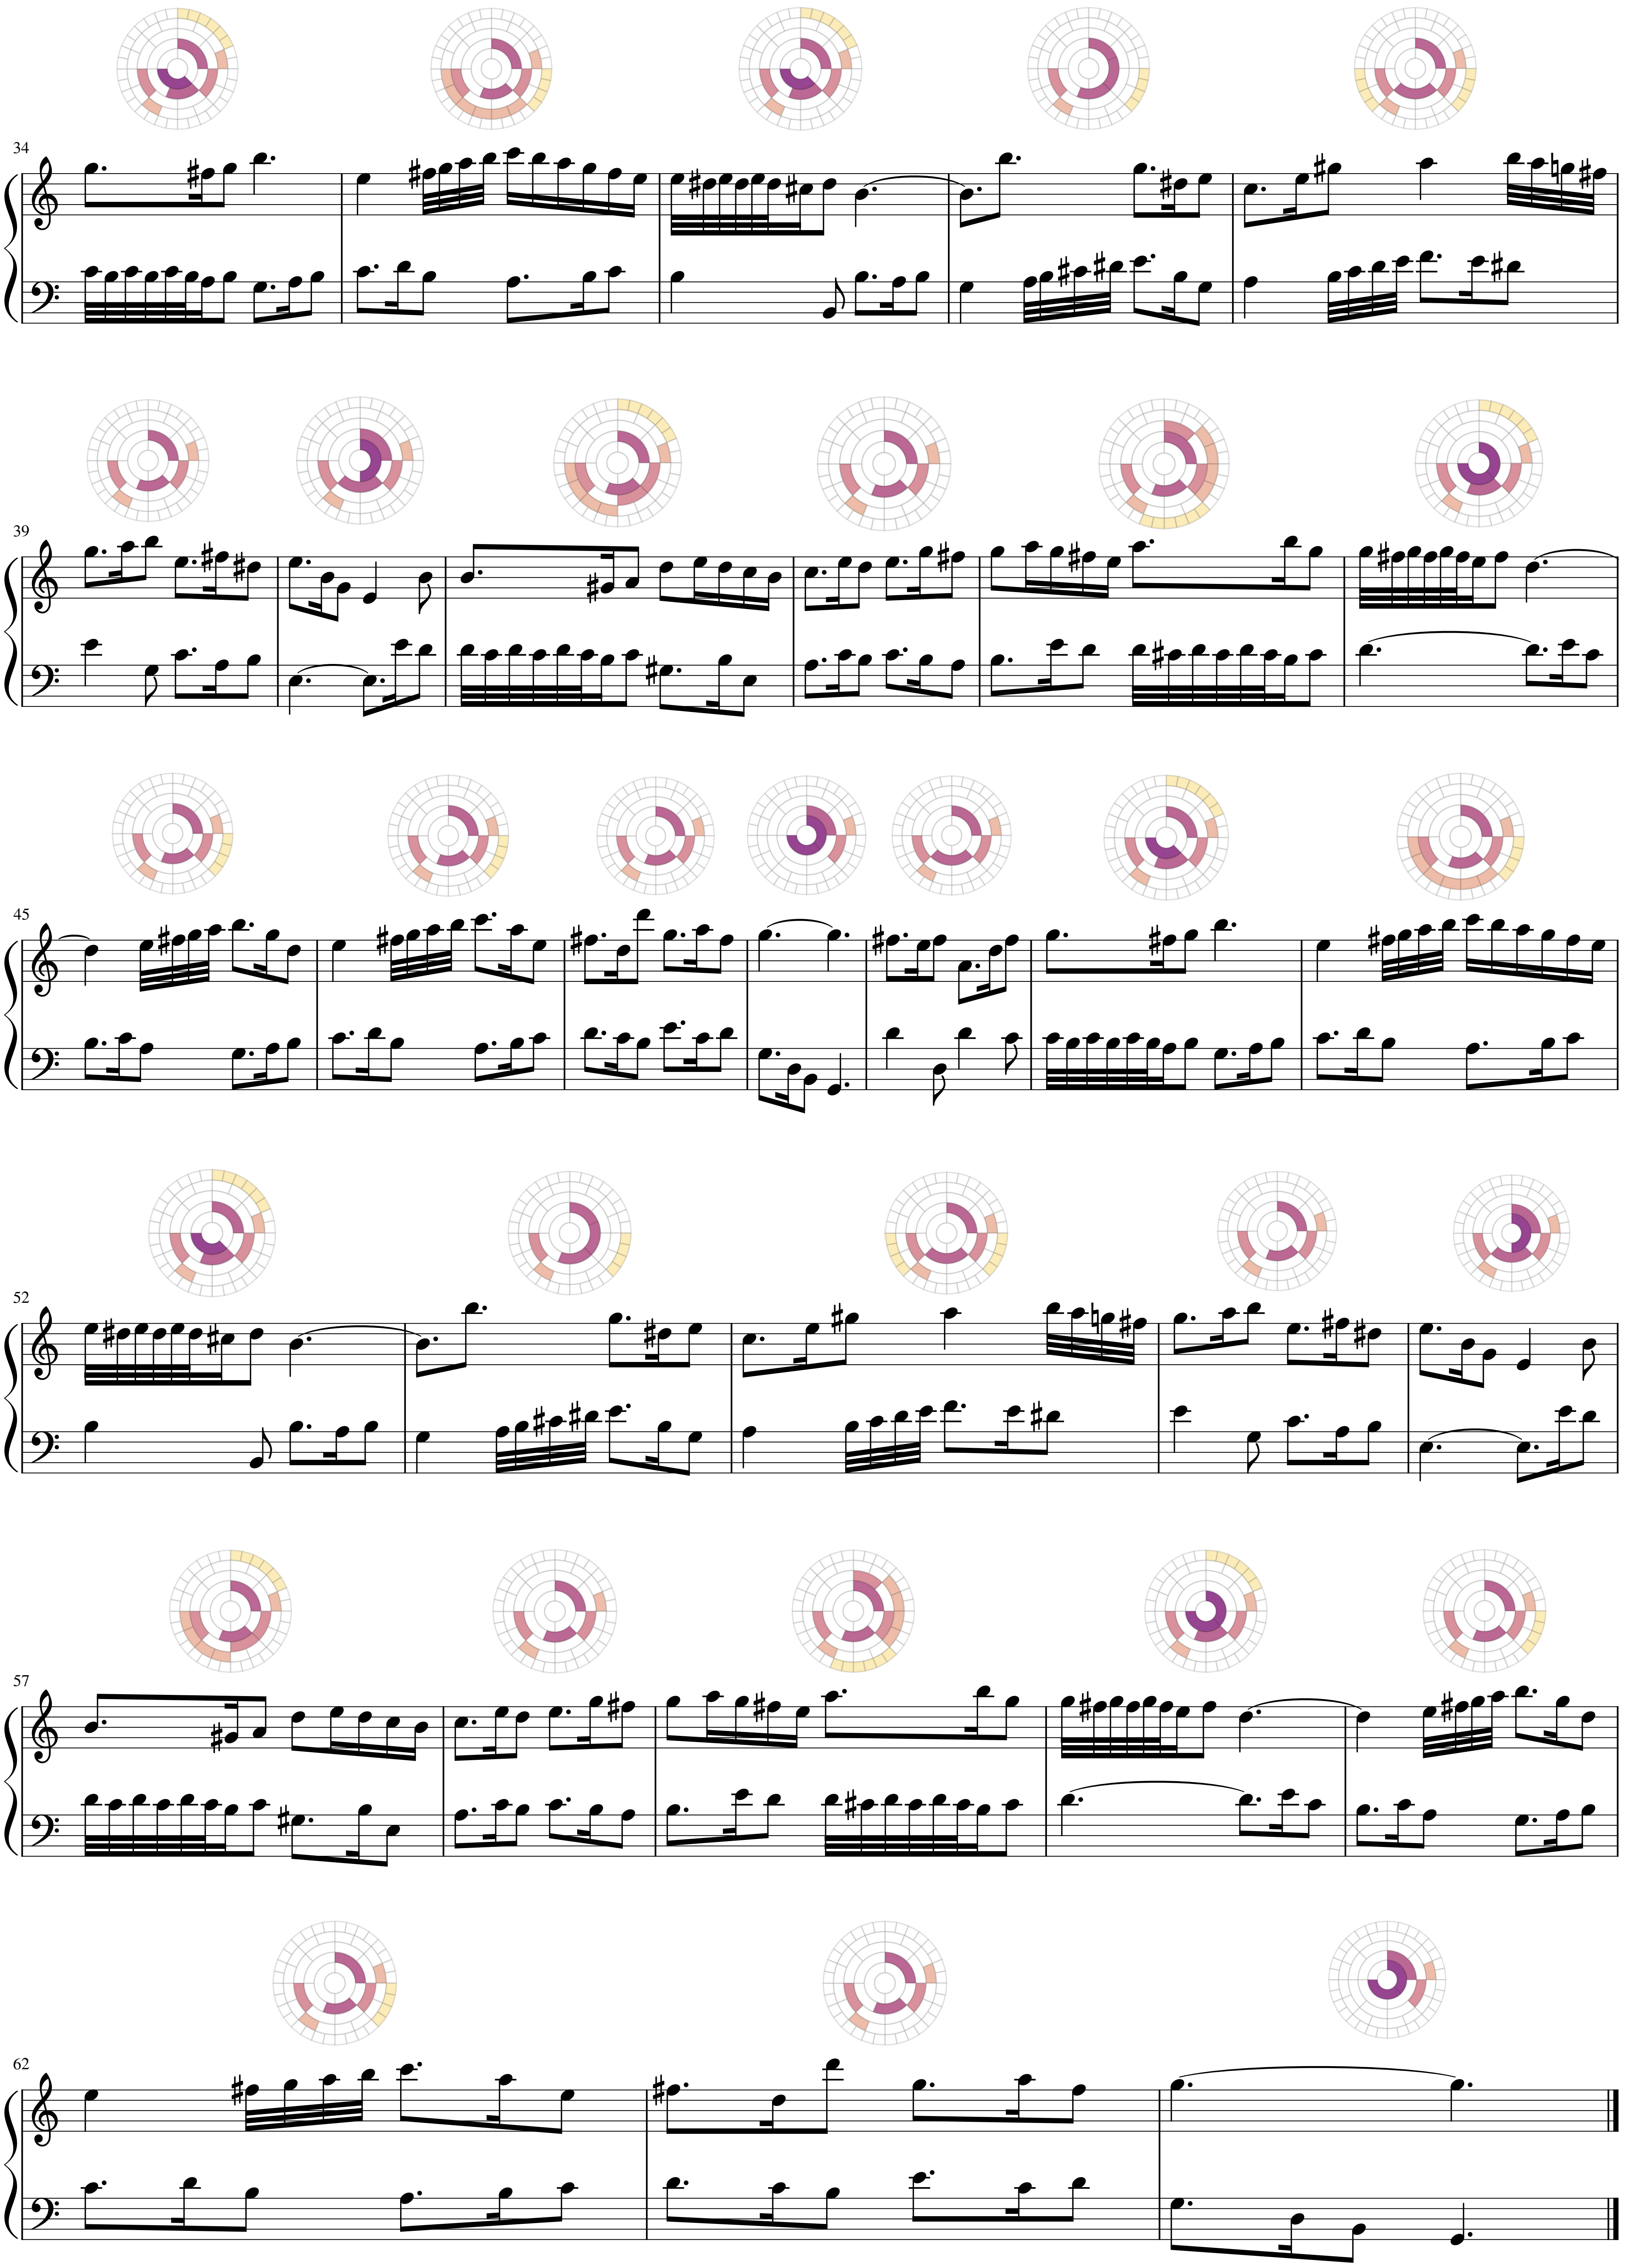
34
39
45
52
57
62
