# Supplementary material for: Augmenting Sheet Music with Rhythmic Fingerprints
Source: arXiv:2009.02057 source file (2020-09-04)
Supplement: Supplementary file 3 [file Johann_Sebastian_Bach_-_Goldberg_Variations_-_Aria_MS1_without_Fingerprints.pdf]

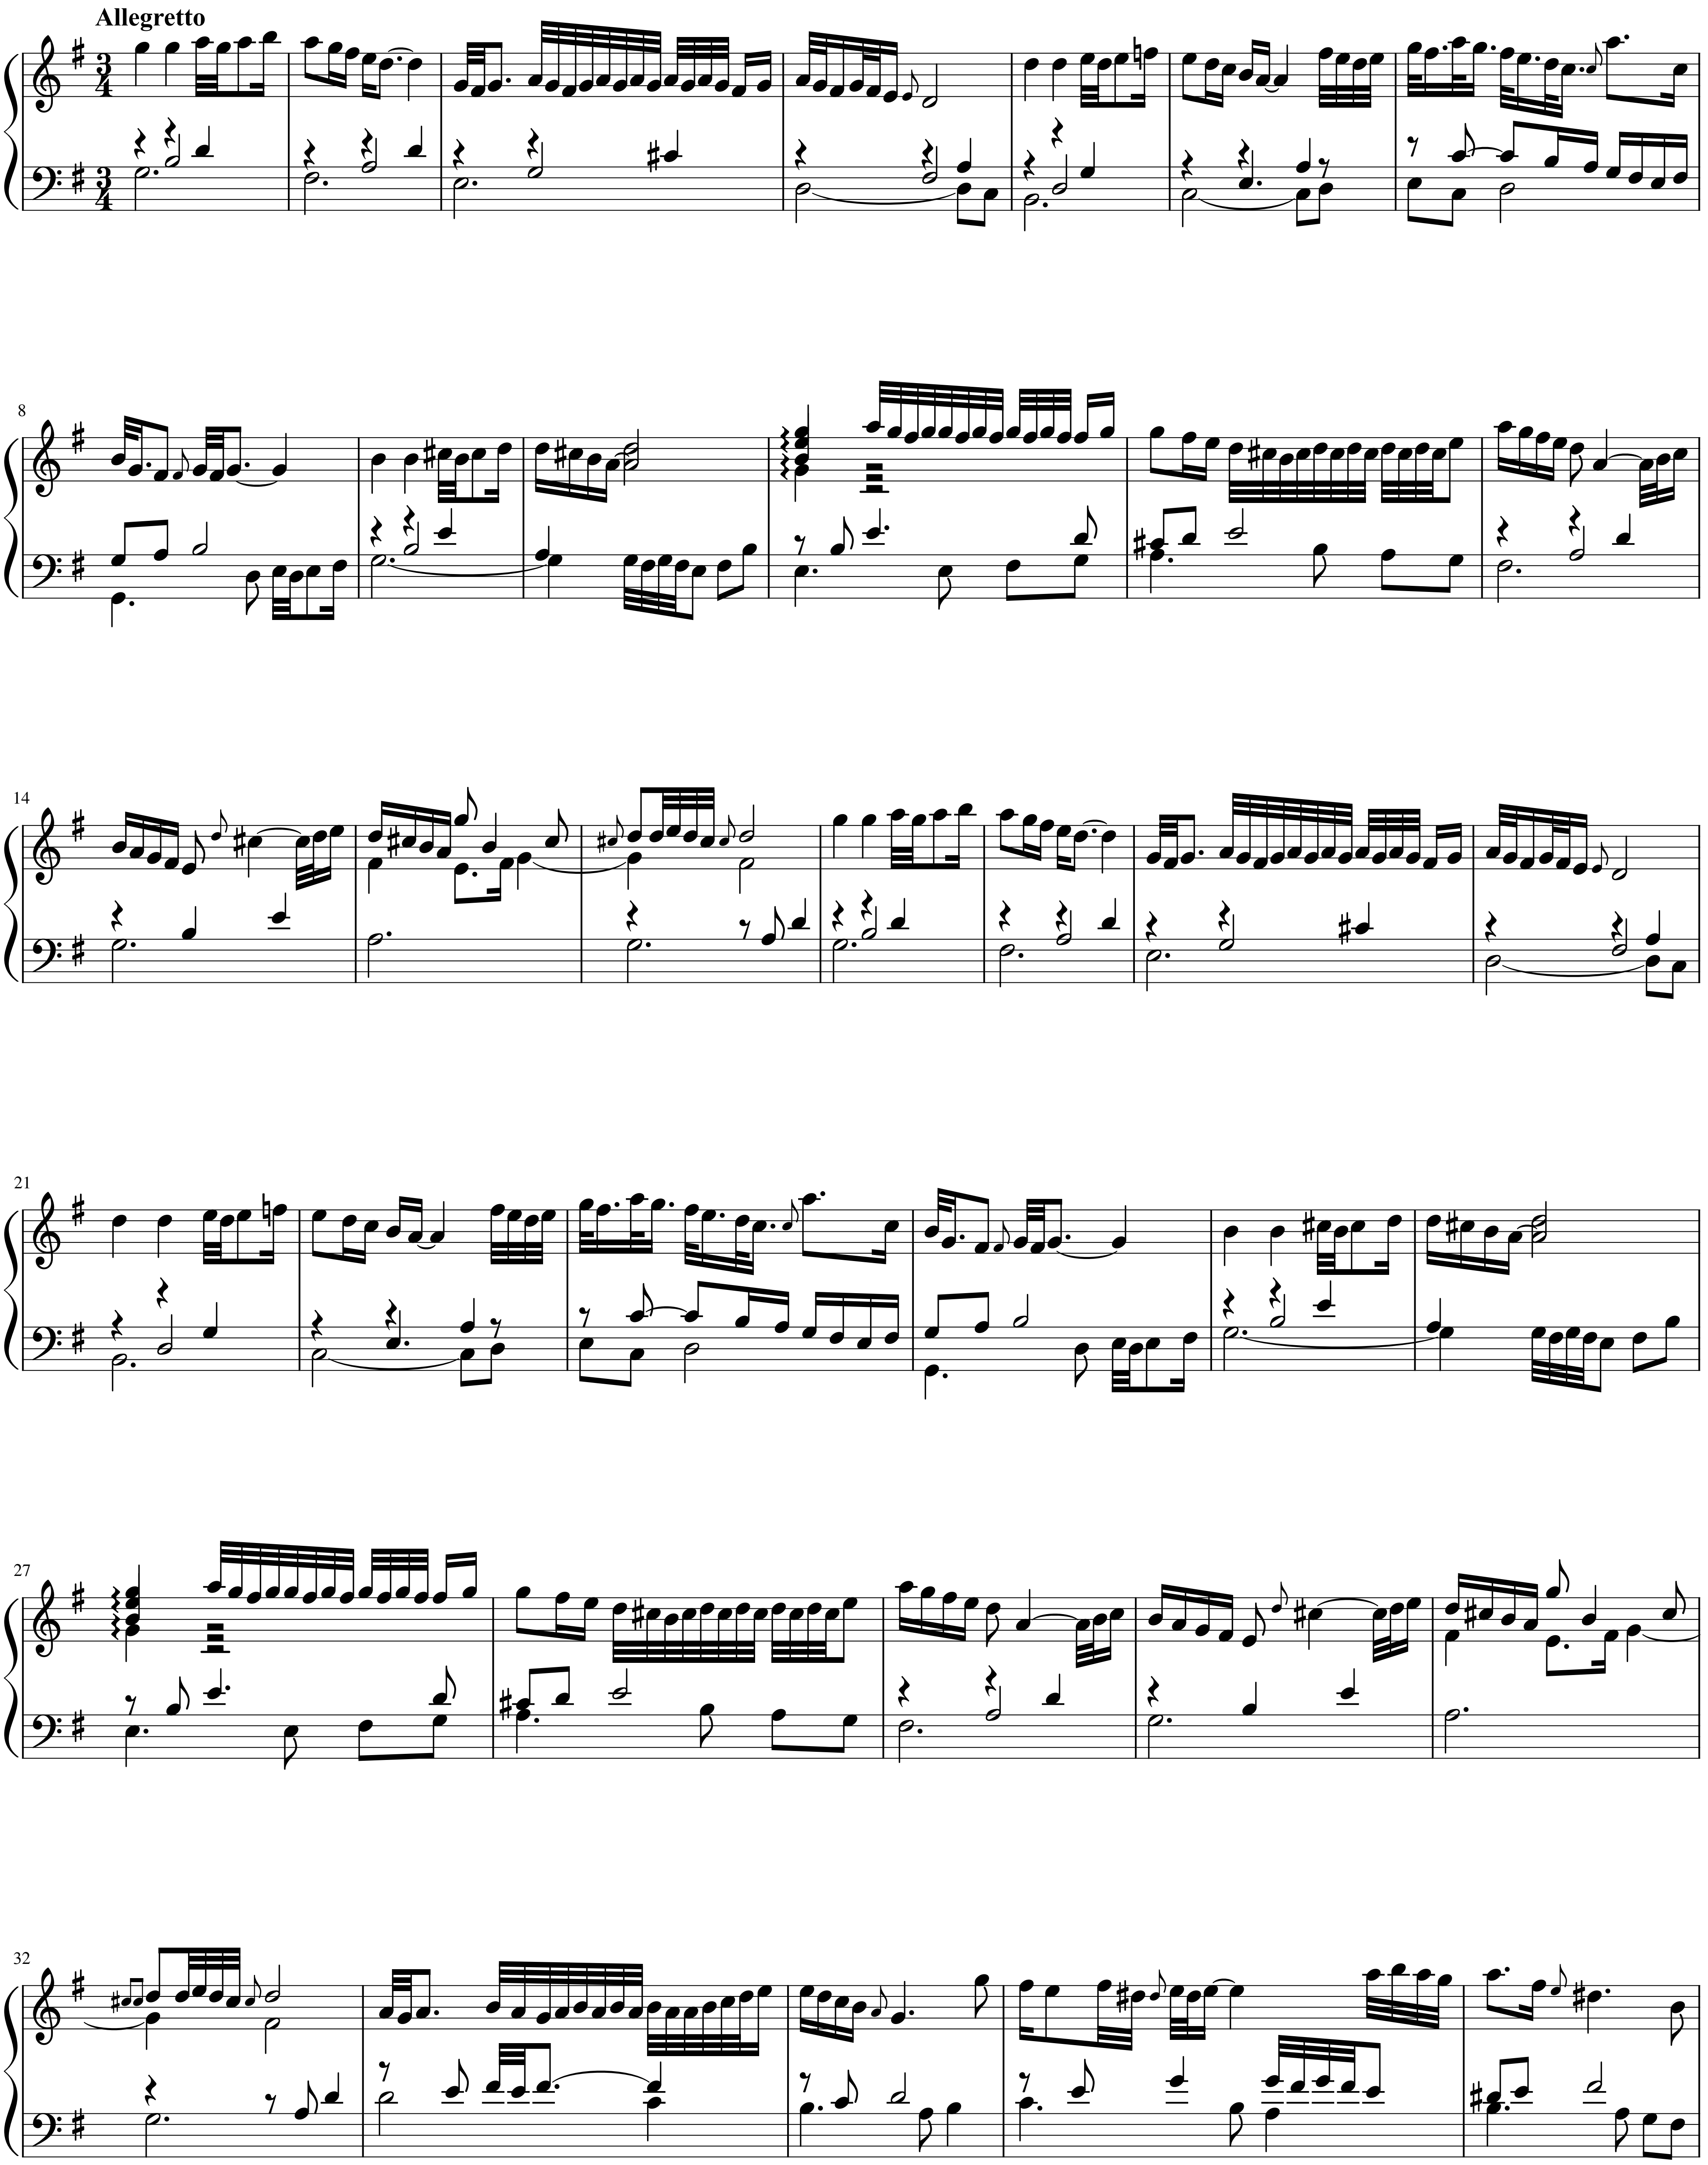
Allegretto
8
14
21
27
32

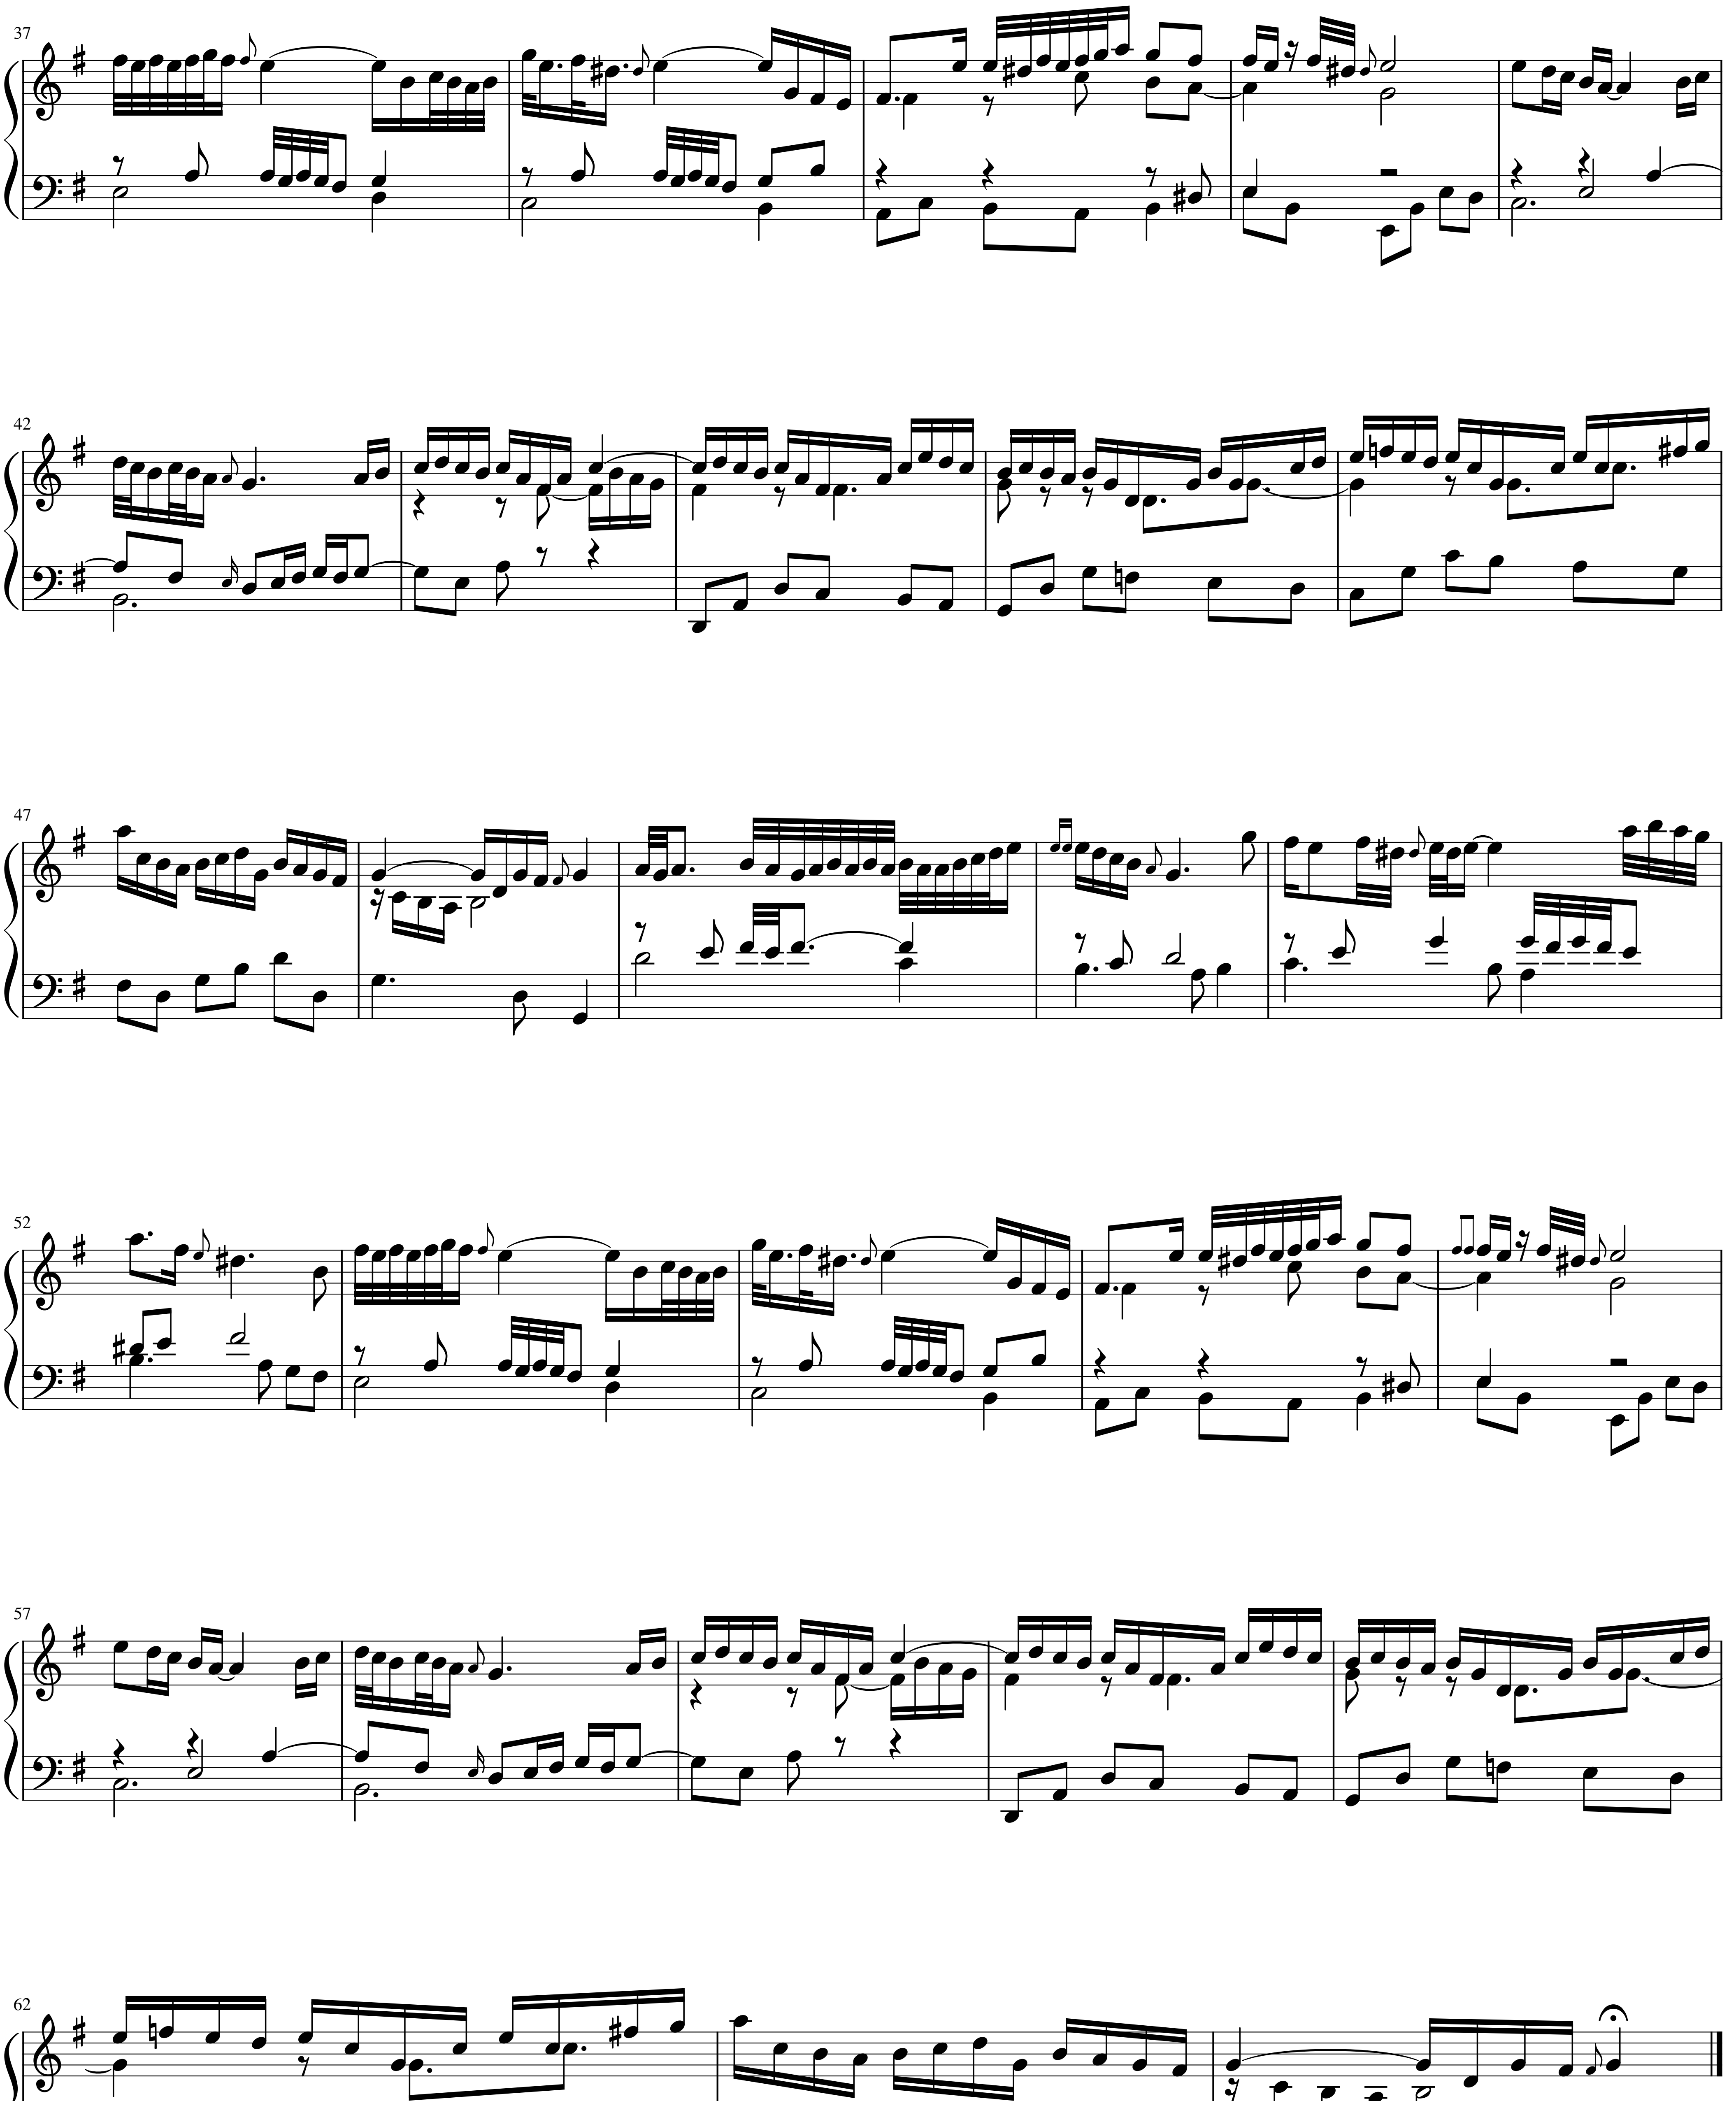
37
42
47
52
57
62
