# Supplementary material for: Augmenting Sheet Music with Rhythmic Fingerprints
Source: arXiv:2009.02057 source file (2020-09-04)
Supplement: Supplementary file 4 [file Johann_Sebastian_Bach_-_Goldberg_Variations_-_Variation_VII_MS2_without_Fingerprints.pdf]

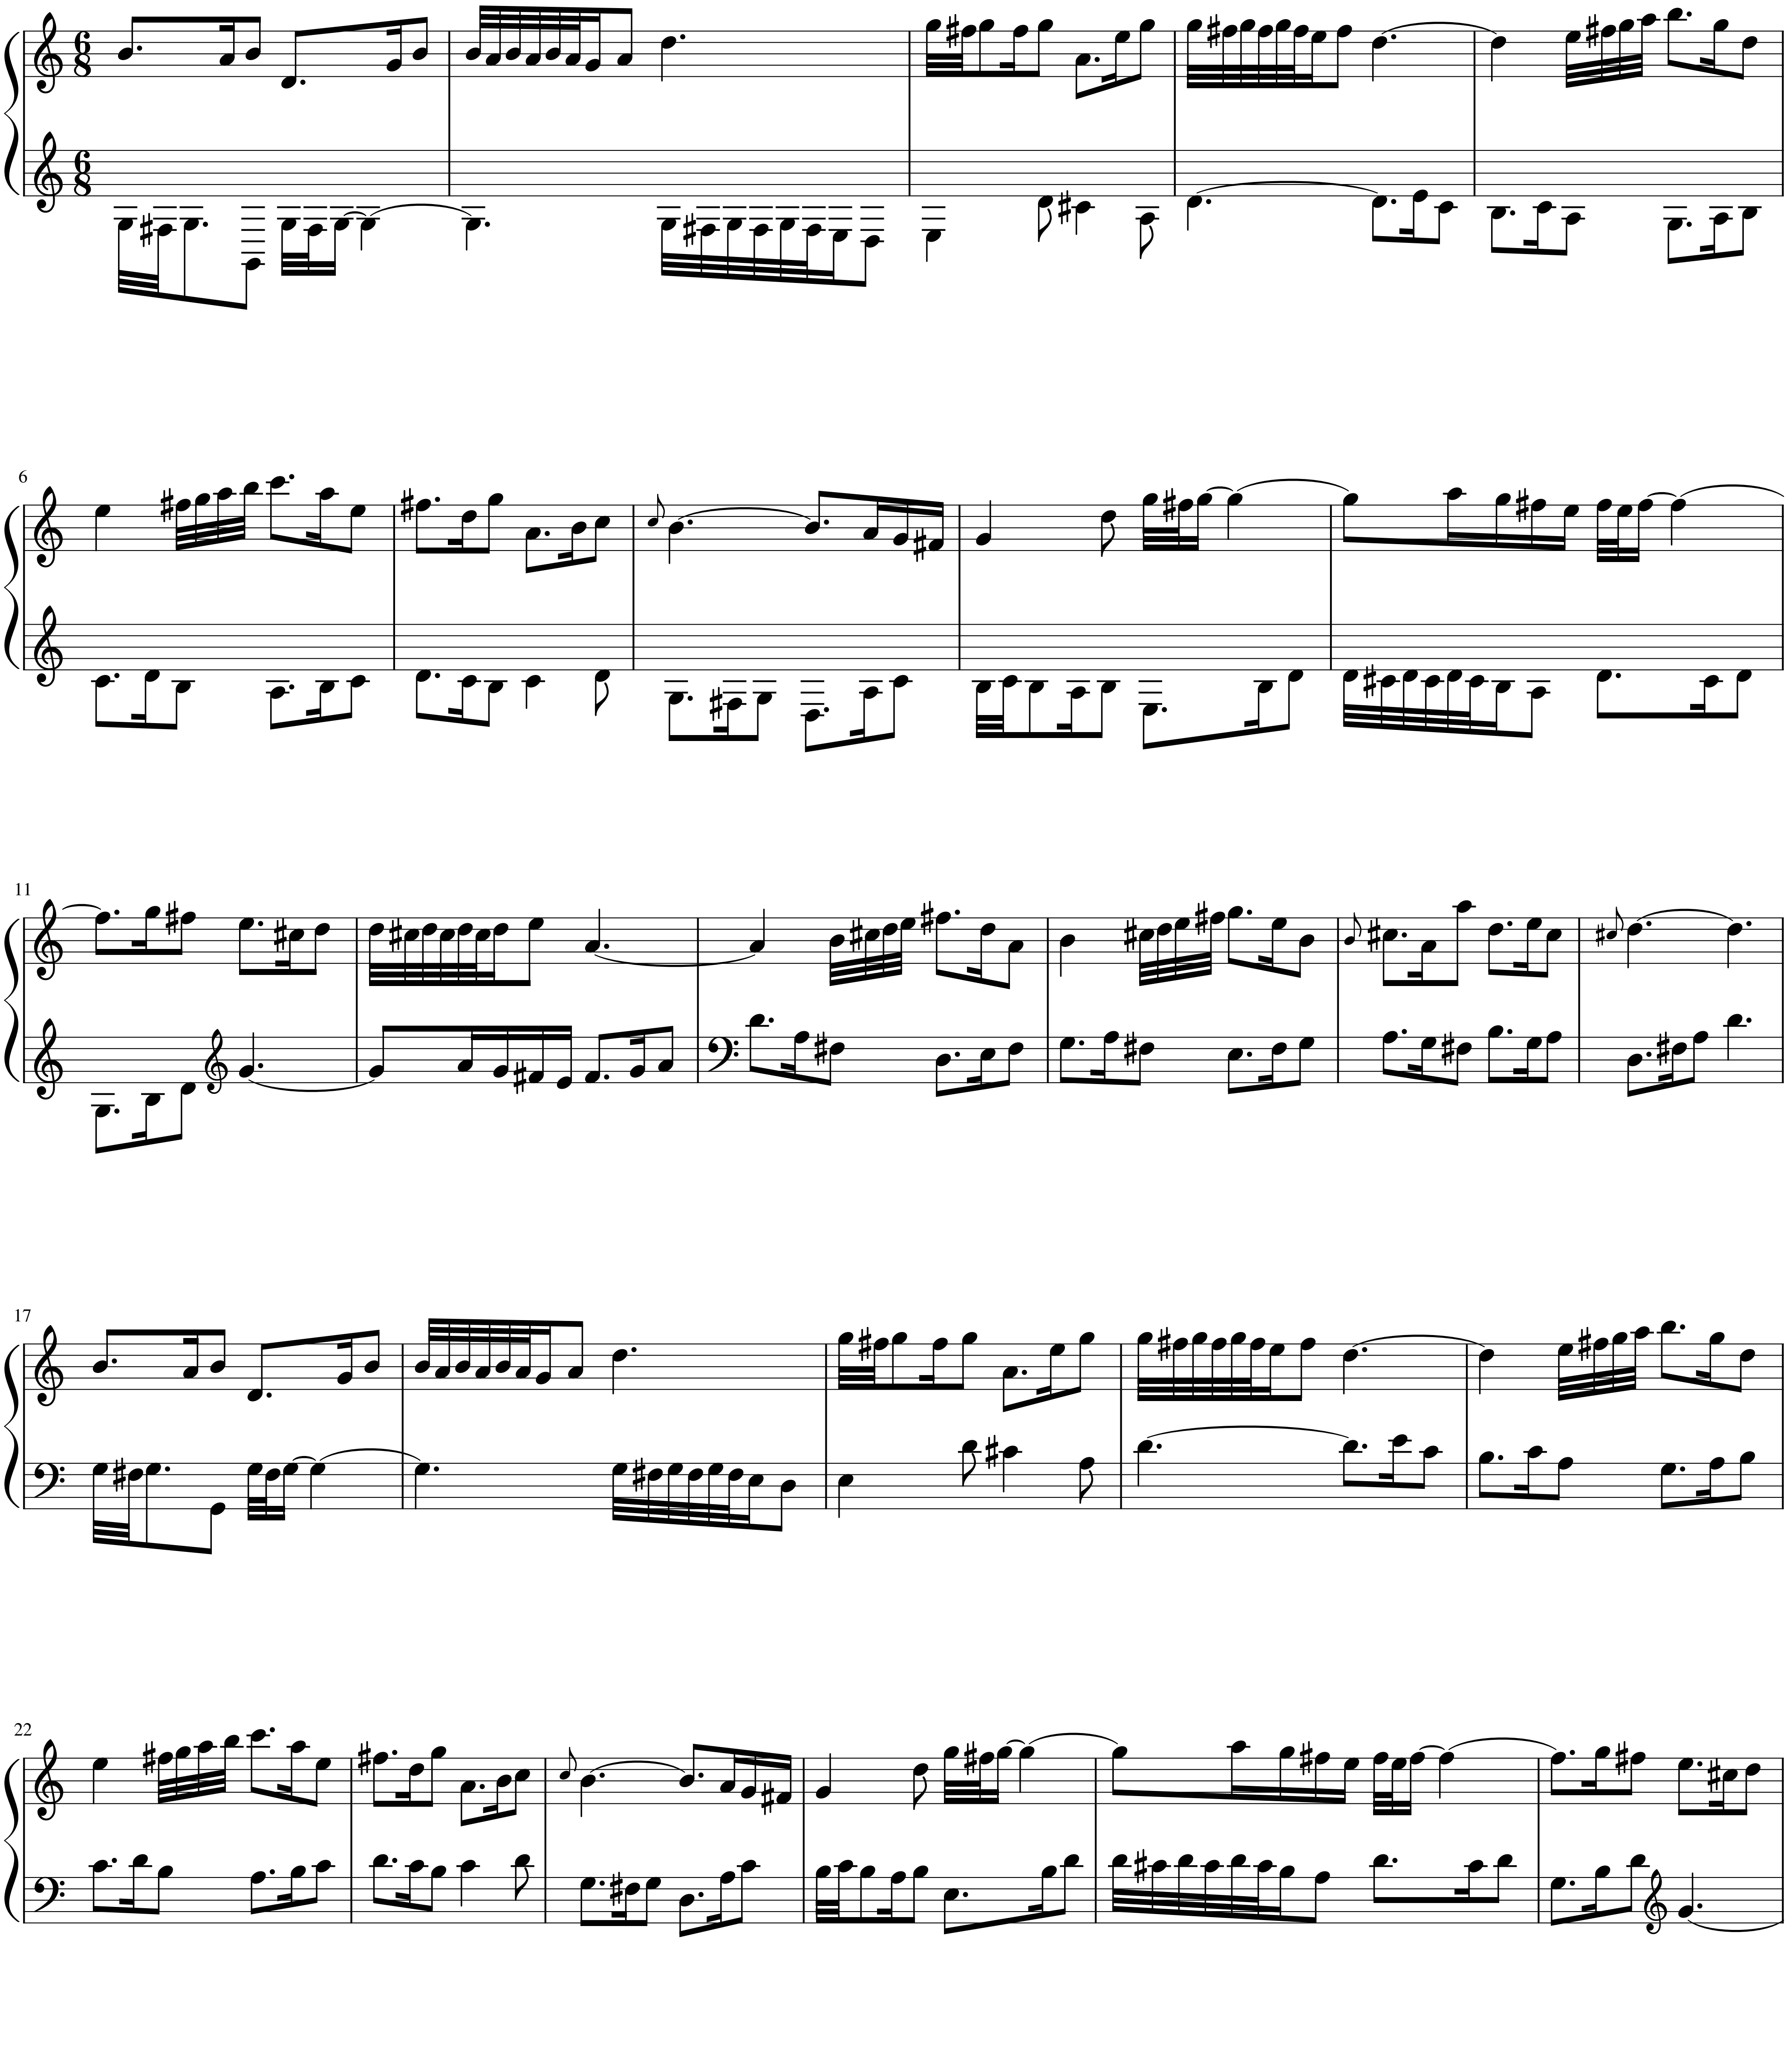

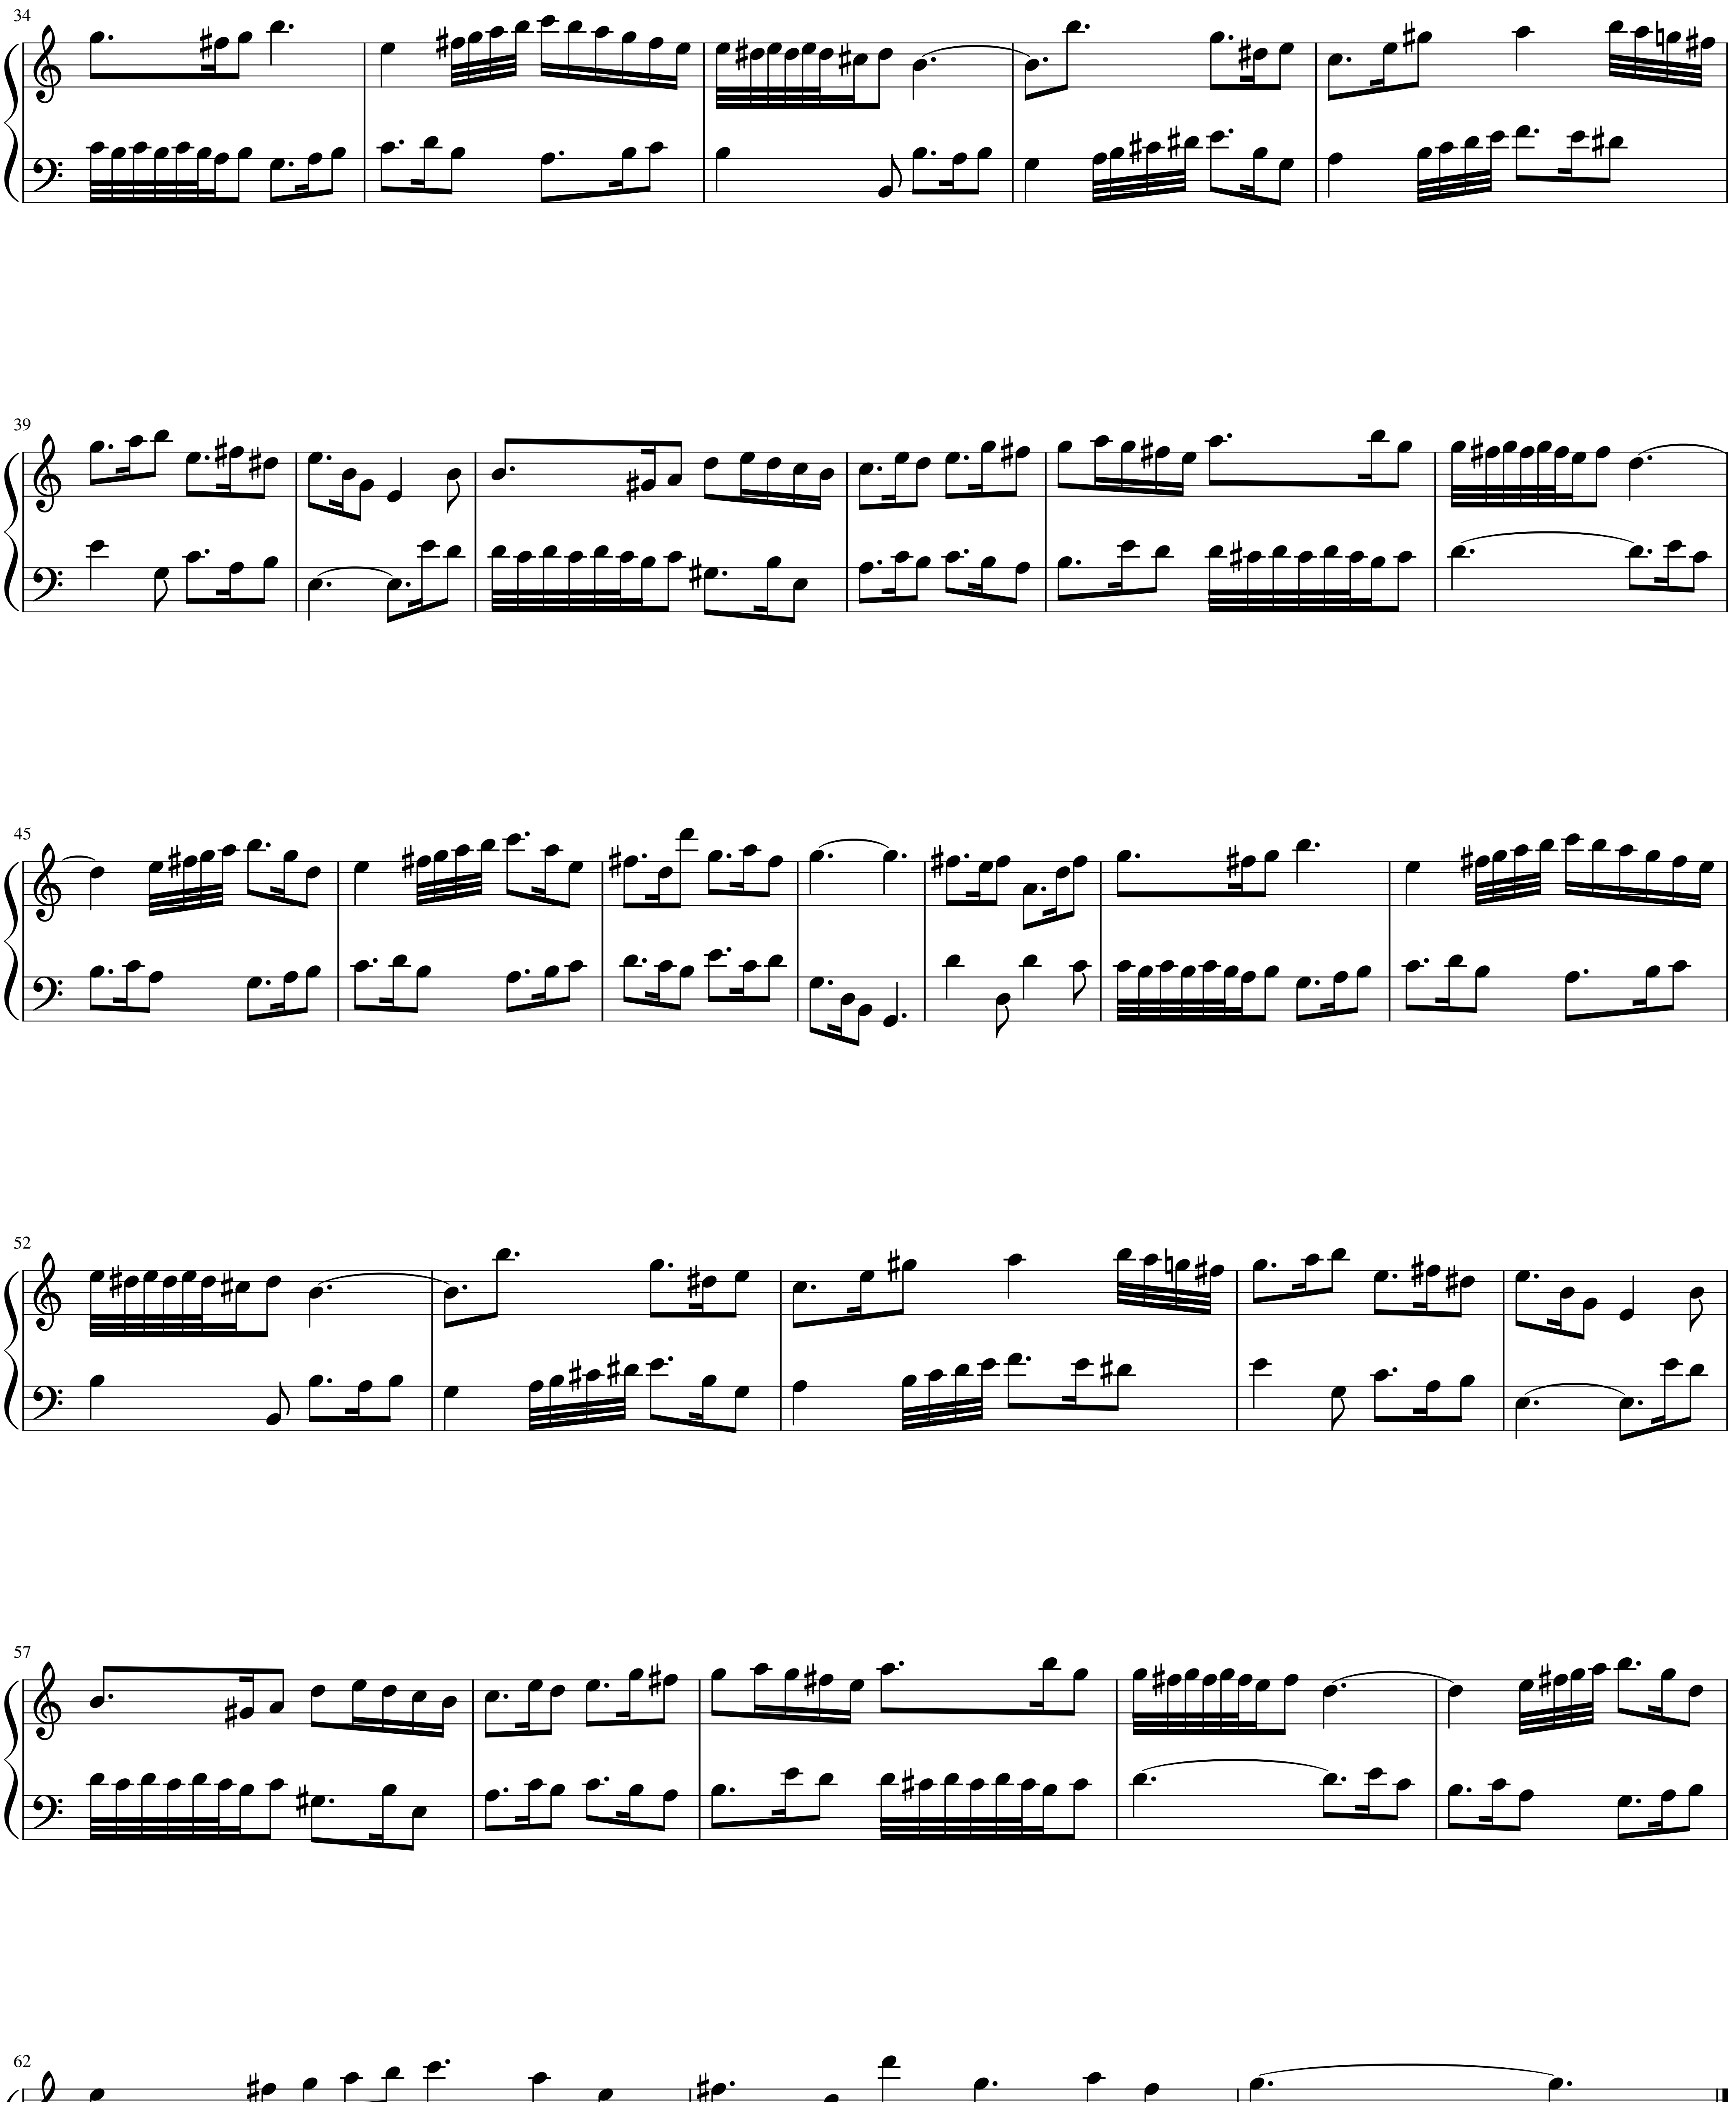
34
39
45
52
57
62
